# Supplementary material for: Extreme-Value Theorems for Optimal Multidimensional Pricing
Source: arXiv:1106.0519 source file (2014-10-26)
Supplement: Supplementary file 1 [file appendix_healthy.tex]

{\color{blue}
\section{Proofs Omitted from Section~\ref{sec:regular}}\label{appendix:regularbounding}
\subsection{Properties of Regular Distributions}\label{sec:regconcavity}
If $F$ is a differentiable continuous regular distribution, it is not hard to see the following: if $f(x)=0$ for some $x$, then $f(x')=0$ for all $x'\geq x$ (as otherwise the definition of regularity would be violated.) Hence, if $X$ is a random variable distributed according to $F$, it must be that $f(x)>0$ for $x\in[u_{min}^{X},u_{max}^{X}]$. So we can define $F^{-1}$ on $[u_{min}^{X},u_{max}^{X}]$, and it will be differentiable, since $F$ is differentiable and $f$ is non-zero. Now we can make the following definition, capturing the revenue of a seller who prices an item with value distribution $F$, so that the item is bought with probability exactly $q$.

\begin{definition}[Revenue Curve]
    For a differentiable continuous regular distribution $F$, define $R_F: [0,1] \rightarrow \mathbb{R}$ as follows
    $$R_F(q) =q\cdot F^{-1}(1-q).$$
\end{definition}
The following is well-known. We include its short proof for completeness.
\begin{lemma}\label{lem:regconcavity}
    If $F$ is regular, $R_F(q)$ is a concave function on $(0,1]$.
\end{lemma}
\begin{proof}
    Take the derivative of $R_F(q)$,
    $$R_F'(q) = F^{-1}(1-q)-{q\over f\big{(}F^{-1}(1-q)\big{)}}$$
    $F^{-1}(1-q)$ is monotonically non-increasing. Then since $F$ is regular, $R_F'(q)$ is  monotonically non-increasing. Thus, $R_F(q)$ is concave.
\end{proof}

\begin{lemma}\label{lem:reglittlegain}
    For any regular distribution $F$, if $q\leq {p}$, where $p\in (0,1)$, then for any $\tilde{q}\leq q$,
    $$R_F(\tilde{q})\leq {1\over 1-p}R_{F}(q).$$ 
\end{lemma}
\begin{proof}
    Since $q\in[\tilde{q},1)$, there exists a $\lambda\in(0,1]$, such that 
    $$\lambda\cdot\tilde{q}+(1-\lambda)\cdot 1=q.$$
    Thus, $\lambda = {1-q\over 1-\tilde{q}}\geq {1-{p}\over 1} = 1-{p}.$
    From Lemma~\ref{lem:regconcavity}, we know that $R_F(x)$ is concave, thus we have the following,
    $$R_F(q)=R_F\big{(}\lambda\cdot\tilde{q}+(1-\lambda)\cdot1\big{)}\geq\lambda\cdot R_F(\tilde{q})+(1-\lambda)\cdot R(1).$$ 
    Since $R_F(1)\geq 0$, $R_F(q)\geq \lambda\cdot R_F(\tilde{q})\geq (1-p)R_F(\tilde{q})$.
    
    Thus, $R_F(\tilde{q})\leq {1\over 1-p}R_{F}(q)$.
\end{proof}    

\begin{corollary}\label{cor:reglittlegain}
        For any regular distribution $F$, if $q\leq {1\over n^{3}}$,  then for any $\tilde{q}\leq q$,
$$R_F(\tilde{q})\leq {n^{3}\over n^{3}-1}R_{F}(q).$$ 
\end{corollary}
\subsection{Restricting the Prices for the Original Distributions}\label{sec:regrestrictprice}
From now on, we only consider the case that $n$ is greater than some absolute constant.\footnote {If $n$ is smaller than the constant, we can add dummy items, which are items that always have value $0$. This will not change the solution at all.}

First we demonstrate a property of the ``center'' $\alpha$.
\begin{proposition}\label{prop:regalpha}
$\alpha\geq \max_i \alpha_{n^3}^{(i)}.$ 
\end{proposition}
\begin{proof}
Since $1/n^{3}\leq 1-c_{2}\leq 1-F(a_{i})\leq 1-c_{1}$, according to Lemma~\ref{lem:reglittlegain}, ${1\over c_{1}}\cdot a_{i}\cdot\big{(}1-F_{i}(a_{i})\big{)}\geq \alpha_{n^{3}}^{(i)}/n^{3}$. Thus, $\alpha\geq {n^{3}\over c_{1}}\cdot \Big{[}a_{i}\cdot \big{(}1-F_{i}(a_{i})\big{)}\Big{]}\geq \alpha_{n^{3}}^{(i)}$.
\end{proof}

Now, we are ready to show that we can restrict all the prices to be smaller than $n^{2}\alpha$ without losing much revenue.
\begin{lemma}\label{lem:regtrunchigh}
    If for any price vector $P$, which has some price greater than $n^2\alpha$, we can construct a new price vector $P'$, such that $\forall\ i$  $p'_i\leq n^2\alpha$, and $\mathcal{R}_{P'}\geq \mathcal{R}_{P}-{5\mathcal{R}_{OPT}\over n}$.
\end{lemma}
\begin{proof}
    For each $i$ that $p_i> n^2\alpha$, we will construct a new $p_i'$, which is smaller than $\alpha$. We will show that no matter what the other prices are, changing $p_i$ to $p_i'$ will only cause at most $O({\mathcal{R}_{OPT}\over n^2})$ loss in revenue. Since we perform this transformation for at most $n$ times, we can argue that the total loss is bounded by $O({\mathcal{R}_{OPT}\over n})$.
    
    WLOG, we assume $p_n> n^2\alpha$. Let $p_n'$ to $(n^2-1)\alpha$.
    \begin{enumerate}
        \item We first bound the loss in the contribution to revenue from item $n$ when the price is $p_n$ and $p_n'$.
        \begin{itemize}
            \item We claim that the contribution to revenue from item $n$ under $p_n'$ is at least $$p_n'\cdot \Pr[v_n\geq n^2\alpha]\cdot(1-{1\over n^2}).$$
            This is because when $v_n\geq n^2\alpha$, the gap $v_n-p_n'$ is at least $\alpha$. If $n$ is not the winner, then there exists some $i\in[n-1]$, who has a larger gap. But
            \begin{align*}
                \Pr[\exists\ i\in[n-1]\ has\ gap\ larger\ than\ \alpha]\leq \Pr[\exists\ i\in[n-1]\ v_i\geq\alpha]\leq {1\over n^3}\cdot n = {1\over n^2}
                \end{align*}
                So with probability at least $1-{1\over n^2}$, $n$ will be the winner.
            \item We claim that the contribution to revenue from item $n$ under $p_n$ is at most $p_n$ is at most 
            $${n^3\over n^3-1}\cdot n^2\alpha\cdot \Pr[v_n\geq n^2\alpha].$$
            We know that the contribution is at most $p_n\cdot \Pr[v_n\geq p_n]=R_{F_{n}}(\Pr[v_n\geq p_n])$. Since $\Pr[v_n\geq p_n]\leq \Pr[v_n\geq n^2\alpha]\leq \Pr[v_m\geq \alpha_{n^3}^{(n)}]=1/n^3$, by Corollary~\ref{cor:reglittlegain}, we know that 
            $$R_{F_{n}}(\Pr[v_n\geq p_n])\leq{n^3\over n^3-1}\cdot R_{F_{n}}(\Pr[v_n\geq n^2\alpha])={n^3\over n^3-1}\cdot n^2\alpha\cdot \Pr[v_n\geq n^2\alpha].$$  
        \end{itemize}
        So the loss from the contribution from item $n$ is at most 
        \begin{align*}
            &{n^2\alpha\cdot \Pr[v_n\geq n^2\alpha]\over n^3-1}+{p_n'\cdot \Pr[v_n\geq n^2\alpha]\over n^2}\\+&n^2\alpha\cdot \Pr[v_n\geq n^2\alpha]-p_n'\alpha\cdot \Pr[v_n\geq n^2\alpha]\\ \leq &{2\mathcal{R}_{OPT}\over n^2}+\alpha\cdot\Pr[v_n\geq n^2\alpha]
        \end{align*}
        $n^2\alpha\cdot \Pr[v_n\geq n^2\alpha]$ is smaller than $\mathcal{R}_{OPT}$, because we can achieve it by setting $p_n = n^2\alpha$ and all other $p_i=+\infty$.
        Again, by Corollary~\ref{cor:reglittlegain} we know that $n^2\alpha\Pr[v_n\geq n^2\alpha]\leq {n^3\over n^3-1}\cdot \alpha\cdot \Pr[v_n\geq \alpha]$. Therefore, 
        $$\alpha\cdot\Pr[v_n\geq n^2\alpha] \leq {n^3\over n^3-1}\cdot {\alpha\cdot \Pr[v_n\geq \alpha]\over n^2}\leq {2\mathcal{R}_{OPT}\over n^2}.$$
        So the loss is at most ${4\mathcal{R}_{OPT}\over n^2}$.
        
        \item Now we bound the loss in the contribution from items in $[n-1]$
        \begin{itemize}
            \item When item $n$'s price is $p_n$, the contribution from items in $[n-1]$ is no greater than the total revenue when we ignore item $n$ (by setting the price for item $n$ to $+\infty$). Since in this case, any $i\in[n-1]$ has at least the same probability of being the winner.
            \item When item $n$'s price is $p_n'$, $\Pr[v_n\geq p_n']\leq {1\over n^3}$. So with probability $1-{1\over n^3}$, the item that has the largest positive gap among items $1$ to $n-1$ is the winner. This means with probability $1-{1\over n^3}$, we can ignore item $n$. Since the distributions are independent, the contribution from items in $[n-1]$ is at least $1-{1\over n^3}$ of the seller's total revenue when we ignore item $n$. 
        \end{itemize}
        So the total difference is $\mathcal{R}_{OPT}\over n^3$ at most.
    \end{enumerate}
    To sum up, the total loss is smaller than $5\mathcal{R}_{OPT}\over n^2$. If we perform this transformation for $n$ times, the total loss is at most $5\mathcal{R}_{OPT}\over n$.
\end{proof}

{To complement this lemma, we have Lemma~\ref{lem:trunclow}, which states that we can set prices below $\alpha/n^4$ to $\alpha/n^4$ and only lose $\alpha/n^4\leq{\max_{i} \Big{[}a_{i}\cdot \big{(}1-F_{i}(a_{i})\big{)}\Big{]}\big{/} c_{1}}\leq \mathcal{R}_{OPT}/c_{1}n$. Now we know if we restrict the prices to be in $[\alpha/n^4, n^2\alpha]$,the revenue decreases for at most $O({\mathcal{R}_{OPT}\over n})$.

\subsection{Bounding the Support of the Distributions}\label{sec:regboundingdistribution}
To establish Theorem~\ref{thm:regreduction}, we need to argue that if we only consider the restricted prices, we can also bound the support of the value distributions.

\begin{lemma}\label{lem:regboundinghigh}
   Given a collection of random variables $\mathcal{V}=\{v_i\}_{i\in[n]}$ that are \text{regular}, let us define a new collection of random variables $\hat{\mathcal{V}}=\{\hat{v}_i\}_{i\in[n]}$ via the following coupling: for all $i\in [n]$, if $v_i\leq 2n^{4}\alpha$, set $\hat{v}_i=v_i$, otherwise set $\hat{v}_i = 2n^{4}\alpha$, where $\alpha$ is the same as defined in Lemma~\ref{lem:regtrunchigh}. Then, for any price vector $P\in[\alpha/n^4, n^2\alpha]^{n}$, $|\mathcal{R}_{P}(\mathcal{V})-{\mathcal{R}}_{P}(\hat{\mathcal{V}})|\leq {\mathcal{R}_{OPT}(\mathcal{V})\over c_{1} n}$.% where $\mathcal{R}_P$ and $\mathcal{R}}_P$ are respectively the revenues of seller when the buyer's values are distributed as $\{v_i\}_{i\in[n]}$ and as $\{\hat{v}_i\}_{i\in[n]}$.
\end{lemma}
\begin{proof}
    By Corollary~\ref{cor:reglittlegain}, we know that for every $i$, ${\alpha_{n^7}^{(i)}\over n^7}\leq {n^3\over n^3-1}\cdot {\alpha_{n^3}^{(i)}\over n^3}\leq {n^3\over n^3-1}\cdot{\alpha\over n^3}$. So $2n^4\alpha\geq \alpha_{n^7}^{(i)}$.
    The probability for the event that there exists an $i$ such that $v_i\geq 2n^4\alpha$ is no greater than $n/n^7=1/n^6$. Thus the difference of contribution to revenue from this event is no greater than ${n^2\alpha\over n^6} = {\alpha\over n^4}\leq {\max_{i} \Big{[}a_{i}\cdot \big{(}1-F_{i}(a_{i})\big{)}\Big{]}\big{/} c_{1}}\leq {\mathcal{R}_{OPT}\over c_{1}n}$.

    If $\forall i$ $v_{i}\leq 2n^{4}\alpha$, then $\hat{v}_{i}=v_{i}$ for all $i$. So the contribution to the revenue is the same in both cases.
    
    Thus, $|\mathcal{R}_{P}-\hat{\mathcal{R}}_{P}|\leq {\mathcal{R}_{OPT}\over c_{1}n}$
\end{proof}

On the other hand, according to Lemma~\ref{lem:boundinglow}, we can create another collection of mutually independent random variables $\tilde{\mathcal{V}}=\{\tilde{v}_{i}\}_{i\in[n]}$ based on $\hat{\mathcal{V}}$ defined in Lemma~\ref{lem:regboundinghigh}, such that $\forall i$ $\tilde{v}_{i}$ is supported on $[{\alpha\over 2n^4},2n^{4}\alpha]$, and the seller's revenue is unchanged under any price vector in $[\alpha/n^4, n^2\alpha]^{n}$, no matter the value distributions are $\hat{\mathcal{V}}$ or $\tilde{\mathcal{V}}$. 
}

\subsection{Restricting the Prices for the Bounded Distributions}\label{sec:regrestrictpricebounded}

In this section, we will show that for the value distributions $\tilde{\mathcal{V}}=\{\tilde{v}_{i}\}_{i\in[n]}$, which are supported on the common interval $[{\alpha\over 2n^4},2n^{4}\alpha]$, the revenue will only be slightly affected if we restricted the price vector to be in $[0, n^{2}\alpha]^{n}$. The proof of this Lemma is essentially the same as its counterpart Lemma~\ref{lem:regtrunchigh}.

\begin{lemma}\label{lem:regboundedtrunchigh}
Given a collection of mutually independent random variables $\mathcal{V}=\{v_i\}_{i\in[n]}$ that are regular, let us define a new collection of random variables $\tilde{\mathcal{V}}=\{\tilde{v}_i\}_{i\in[n]}$ via the following coupling: for all $i\in [n]$, set  $\tilde{v}_i={\alpha\over 2n^4}$ if $v_i < {\alpha\over n^4}$, set $\tilde{v}_i=2n^{4}\alpha$ if $v_i\ge 2n^{4}\alpha$, and set $\tilde{v}_i=v_i$ otherwise, where $\alpha\geq \max_{i}\alpha_{n^{3}}^{(i)}$ (Defined on  $\{v_i\}_i$). If for any price vector $P$, which has some price greater than $n^2\alpha$, we can construct a new price vector $P'$, such that $\forall\ i$  $p'_i\leq n^2\alpha$, and 
$${\mathcal{R}}_{P'}(\tilde{\mathcal{V}})\geq {\mathcal{R}}_{P}(\tilde{\mathcal{V}})-{5{\mathcal{R}}_{OPT}(\tilde{\mathcal{V}})\over n},$$
% where $\mathcal{R}_P$ and $\tilde{\mathcal{R}}_P$ are respectively the revenues of seller when the buyer's values are distributed as $\{v_i\}_{i\in[n]}$ and as $\{\tilde{v}_i\}_{i\in[n]}$. $\tilde{\mathcal{R}}_{OPT}= \max_{P} \tilde{\mathcal{R}}_{P}$.
\end{lemma}

\begin{proof}
    For each $i$ that $p_i> n^2\alpha$, we will construct a new $p_i'$, which is smaller than $\alpha$. We will show that no matter what the other prices are, changing $p_i$ to $p_i'$ will only cause at most $O({\mathcal{R}_{OPT}(\tilde{\mathcal{V}})\over n^2})$ loss in revenue. Since we perform this transformation for at most $n$ times, we can argue that the total loss is bounded by $O({\mathcal{R}_{OPT}(\tilde{\mathcal{V}})\over n})$.
    
    WLOG, we assume $p_n> n^2\alpha$. Let $p_n'$ to $(n^2-1)\alpha$.
    \begin{enumerate}
        \item We first bound the loss in the contribution to revenue from item $n$ when the price is $p_n$ and $p_n'$.
        \begin{itemize}
            \item We claim that the contribution to revenue from item $n$ under $p_n'$ is at least $$p_n'\cdot \Pr[\tilde{v}_n\geq n^2\alpha]\cdot(1-{1\over n^2})=p_n'\cdot \Pr[{v}_n\geq n^2\alpha]\cdot(1-{1\over n^2}).$$
            This is because when $\tilde{v}_n\geq n^2\alpha$, the gap $\tilde{v}_n-p_n'$ is at least $\alpha$. If $n$ is not the winner, then there exists some $i\in[n-1]$, who has a larger gap. But
            \begin{align*}
                &\Pr[\exists\ i\in[n-1]\ has\ gap\ larger\ than\ \alpha]\\ \leq &\Pr[\exists\ i\in[n-1]\ \tilde{v}_i\geq\alpha]=\Pr[\exists\ i\in[n-1]\ {v}_i\geq\alpha]\\ \leq& {1\over n^3}\cdot n = {1\over n^2}
                \end{align*}
                So with probability at least $1-{1\over n^2}$, $n$ will be the winner.
            \item We claim that the contribution to revenue from item $n$ under $p_n$ is at most $p_n$ is at most 
            $${n^3\over n^3-1}\cdot n^2\alpha\cdot \Pr[v_n\geq n^2\alpha].$$
            We know that the contribution is at most $p_n\cdot \Pr[\tilde{v}_n\geq p_n]\leq R_{F_{n}}(\Pr[v_n\geq p_n])$, because $\Pr[\tilde{v}_n\geq p_n]\leq \Pr[v_{n}\geq p_{n]}$. Since $\Pr[v_n\geq p_n]\leq \Pr[v_n\geq n^2\alpha]\leq \Pr[v_m\geq \alpha_{n^3}^{(n)}]=1/n^3$, by Corollary~\ref{cor:reglittlegain}, we know that 
            $$R_{F_{n}}(\Pr[v_n\geq p_n])\leq{n^3\over n^3-1}\cdot R_{F_{n}}(\Pr[v_n\geq n^2\alpha])={n^3\over n^3-1}\cdot n^2\alpha\cdot \Pr[v_n\geq n^2\alpha].$$  
        \end{itemize}
        So the loss from the contribution from item $n$ is at most 
        \begin{align*}
            &{n^2\alpha\cdot \Pr[v_n\geq n^2\alpha]\over n^3-1}+{p_n'\cdot \Pr[v_n\geq n^2\alpha]\over n^2}\\+&n^2\alpha\cdot \Pr[v_n\geq n^2\alpha]-p_n'\alpha\cdot \Pr[v_n\geq n^2\alpha]\\ \leq &{2\tilde{\mathcal{R}}_{OPT}\over n^2}+\alpha\cdot\Pr[v_n\geq n^2\alpha]
        \end{align*}
        $n^2\alpha\cdot \Pr[v_n\geq n^2\alpha]=n^2\alpha\cdot \Pr[\tilde{v}_n\geq n^2\alpha]$ is smaller than ${\mathcal{R}}_{OPT}(\tilde{\mathcal{V}})$, because we can achieve it by setting $p_n = n^2\alpha$ and all other $p_i=+\infty$.
        Again, by Corollary~\ref{cor:reglittlegain} we know that $n^2\alpha\Pr[v_n\geq n^2\alpha]\leq {n^3\over n^3-1}\cdot \alpha\cdot \Pr[v_n\geq \alpha]$. Therefore, 
        $$\alpha\cdot\Pr[v_n\geq n^2\alpha] \leq {n^3\over n^3-1}\cdot {\alpha\cdot \Pr[v_n\geq \alpha]\over n^2}\leq {2{\mathcal{R}}_{OPT}(\tilde{\mathcal{V}})\over n^2}.$$
        So the loss is at most ${4{\mathcal{R}}_{OPT}(\tilde{\mathcal{V}})\over n^2}$.
        
        \item Now we bound the loss in the contribution from items in $[n-1]$
        \begin{itemize}
            \item When item $n$'s price is $p_n$, the contribution from items in $[n-1]$ is no greater than the total revenue when we ignore item $n$ (by setting the price for item $n$ to $+\infty$). Since in this case, any $i\in[n-1]$ has at least the same probability of being the winner.
            \item When item $n$'s price is $p_n'$, $\Pr[\tilde{v}_n\geq p_n']\leq {1\over n^3}$. So with probability $1-{1\over n^3}$, the item that has the largest positive gap among items $1$ to $n-1$ is the winner. This means with probability $1-{1\over n^3}$, we can ignore item $n$. Since the distributions are independent, the contribution from items in $[n-1]$ is at least $1-{1\over n^3}$ of the total revenue when we ignore item $n$. 
        \end{itemize}
        So the total difference is ${\mathcal{R}}_{OPT}(\tilde{\mathcal{V}})\over n^3$ at most.
    \end{enumerate}
    To sum up, the total loss is smaller than $5{\mathcal{R}}_{OPT}(\tilde{\mathcal{V}})\over n^2$. So if we perform this transformation for $n$ times. The total loss is at most $5{\mathcal{R}}_{OPT}(\tilde{\mathcal{V}})\over n$.
\end{proof}
\subsection{Reduce the Regular Distributions to the $Poly(n)$ Balanced Case} 
\begin{prevproof}{Theorem}{thm:regreduction}
Based on Definition~\ref{def:regalpha}, it is not hard to see that we can compute $\alpha$ in time $O(n)$, if $\mathcal{V}$ is given to us explicitly. If we have oracle access to $\mathcal{V}$, we can still compute $\alpha$ in time polynomial in $n$ and the desired precision. 

Now, let us define $\tilde{\mathcal{V}}$ via the following coupling: for all $i\in [n]$, set  $\tilde{v}_i={\alpha\over 2n^4}$ if $v_i < {\alpha\over n^4}$, set $\tilde{v}_i=2n^{4}\alpha$ if $v_i\ge 2n^{4}\alpha$, and set $\tilde{v}_i=v_i$ otherwise. It is not hard to see that in time polynomial in $n$ and $1/\epsilon$, we can compute the distributions of these variables, if the $\mathcal{V}$ are given explicitly; or construct an oracle for the distributions, if we have oracle access to the distributions of  $\mathcal{V}$.

Let $P$ be the price vector that ${\mathcal{R}}_{P}(\tilde{\mathcal{V}})\geq (1-\epsilon+{(12+4/c_{1})\over n})\cdot {\mathcal{R}}_{OPT}(\tilde{\mathcal{V}})$. According to Lemma~\ref{lem:regboundedtrunchigh}, we can construct $P'\in [0,n^{2}\alpha]^{n}$ efficiently, such that ${\mathcal{R}}_{P'}(\tilde{\mathcal{V}})\geq (1-\epsilon+{(12+4/c_{1})\over n})(1-{5\over n})\cdot {\mathcal{R}}_{OPT}(\tilde{\mathcal{V}})\geq(1-\epsilon+{(6+4/c_{1})\over n})\cdot {\mathcal{R}}_{OPT}(\tilde{\mathcal{V}})$. Then by applying Lemma~\ref{lem:trunclow}, we can construct a new price vector $P''\in[\alpha/n^4, n^2\alpha]^{n}$ in time $O(n)$, such that $${\mathcal{R}}_{P''}(\tilde{\mathcal{V}})\geq (1-\epsilon+{(6+4/c_{1})\over n})\cdot {\mathcal{R}}_{OPT}(\tilde{\mathcal{V}})-{1\over c_{1}n}{\mathcal{R}}_{OPT}(\tilde{\mathcal{V}})\geq (1-\epsilon+{(6+3/c_{1})\over n})\cdot {\mathcal{R}}_{OPT}(\tilde{\mathcal{V}}).$$

Combining Lemma~\ref{lem:regtrunchigh} and~\ref{lem:trunclow}, we know there exists a price vector $\hat{P}\in [\alpha/n^4, n^2\alpha]^{n}$, such that $\mathcal{R}_{\hat{P}}(\mathcal{V})\geq \big{(}1-{(5+1/c_{1})\over n}\big{)}\cdot \mathcal{R}_{OPT}(\mathcal{V})$. By Lemma~\ref{lem:regboundinghigh} and~\ref{lem:boundinglow}, we know that $${\mathcal{R}}_{OPT}(\tilde{\mathcal{V}})\geq {\mathcal{R}}_{\hat{P}}(\tilde{\mathcal{V}})\geq\mathcal{R}_{\hat{P}}(\mathcal{V})-{\mathcal{R}_{OPT}(\mathcal{V})\over c_{1}n}\geq \big{(}1-{(5+2/c_{1})\over n}\big{)}\cdot \mathcal{R}_{OPT}(\mathcal{V}).$$

So ${\mathcal{R}}_{P''}(\tilde{\mathcal{V}})\geq(1-\epsilon+{1\over c_{1}n})\cdot \mathcal{R}_{OPT}(\mathcal{V})$. We can now apply Lemma~\ref{lem:regboundinghigh} and~\ref{lem:boundinglow}, and get $$\mathcal{R}_{P''}(\mathcal{V})\geq{\mathcal{R}}_{P''}(\tilde{\mathcal{V}})-{\mathcal{R}_{OPT}(\mathcal{V})\over c_{1}n} \geq(1-\epsilon)\cdot \mathcal{R}_{OPT}(\mathcal{V}).$$\end{prevproof}% when $n\ge 28/\epsilon$. %If $n< 28/\epsilon$, we can add dummy items to make the number of items $n'=28/\epsilon$, and all the above arguments are still true. 
}
